# Supplementary material for: Simultaneous High-Speed and Low-Dose 4-D STEM Using Compressive Sensing Techniques
Source: arXiv:2309.14055 source file (2023-12-12)
Supplement: Supplementary file 2 [file packages.tex]

\usepackage{amssymb,amsthm,amsmath,array}
\usepackage{graphicx}
\usepackage[caption=false,font=footnotesize]{subfig}
\usepackage{xspace}
\usepackage[sort&compress, numbers]{natbib}
\usepackage{stmaryrd}
\usepackage{xcolor}
% \usepackage{todonotes}
\usepackage{mathtools}
\usepackage{float}
\usepackage{textcomp}

\usepackage{standalone}
\graphicspath{{Figures/}}

%% TIKS
\usepackage{tikz}
% To boost compilation time with TIKZ
\usetikzlibrary{external}
\tikzexternalize % activate!
%% end of boosting
\usetikzlibrary{arrows}
\usepackage{pgfplots}
\pgfplotsset{compat=1.7}

% special font
\newcommand{\fs}{\mathsf}
\newcommand{\cc}{\centering}
\newcommand{\bs}{\boldsymbol}
\newcommand{\bb}{\mathbb}
\newcommand{\cl}{\mathcal}

% New Theorems
\newtheorem{thm}{Theorem}
\newtheorem{lem}{Lemma}
\newtheorem{prop}{Proposition}
\newtheorem{cor}{Corollary}
\newtheorem{definition}{Definition}
\newtheorem{remark}{Remark}

% Misc
\newcommand{\ts}{\textstyle}
\newcommand{\ie}{\emph{i.e.},\xspace}
\newcommand{\eg}{\emph{e.g.},\xspace}
\newcommand{\etal}{\emph{et al.}}
\newcommand{\sq}{\vspace{-2mm}}

%% Comments
\newcommand{\nc}[1]{\textcolor{blue}{#1}}
\newcommand{\AMc}[1]{\textcolor{blue}{\small\textbf{[AM: #1]}}}
\newcommand{\ARc}[1]{\textcolor{red}{\small\textbf{[AR: #1]}}}
\newcommand{\JWc}[1]{\textcolor{orange}{\small\textbf{[JW: #1]}}}
\newcommand{\DNc}[1]{\textcolor{magenta}{\small\textbf{[DN: #1]}}}
\newcommand{\ZBc}[1]{\textcolor{teal}{\small\textbf{[ZB: #1]}}}
